# Supplementary material for: ESP: Exploiting Symmetry Prior for Multi-Agent Reinforcement Learning
Source: arXiv:2307.16186 source file (2023-08-09)
Supplement: Supplementary file 1 [file supplement.pdf]

# Supplementary material for ESP: Exploiting Symmetry Prior for Multi-Agent Reinforcement Learning

**Xin Yu [a], Rongye Shi [a;*], Pu Feng[a], Yongkai Tian[a], Jie Luo[a] and Wenjun Wu [a]**

[a]Beihang University, Beijing, China

## 1 Detailed proof for proposition 1

The Symmetry Markov game proposed in the main content is a subclass of the Markov game endowed with symmetry characterization. The Symmetry Markov game $(N, S, \{A_i\}_{i=1}^n, \{R_i\}_{i=1}^n, T, \Psi, G)$ is a Markov Game that satisfies the conditions of reward invariance and transition invariance. The conditions of reward invariance and the transition invariance are given by:

$$R(s,a) = R(L_g[s], K_g^s[a]), \tag{1}$$

$$T(s,a,s') = T(L_g[s], K_g^s[a], L_g[s']). \tag{2}$$

After recapping the Symmetry Markov game, we provide the proof of proposition 1 in the following. We will use mathematical induction to prove this proposition.

**Proposition 1** (Optimal value equivalence)**.** *Consider a Symmetry Markov game $(N, S, \{A_i\}_{i=1}^n, \{R_i\}_{i=1}^n, T, \Psi, G)$ with an invariant transformation $h = (L_g, K_g)$ where $g \in G$. For any $(s,a) \in \Psi$, it holds that $Q^\star(s,a) = Q^\star(L_g[s], K_g[a])$.*

*Proof.* We define the $m$-step optimal discounted action value function recursively for all $(s,a) \in \Psi$ and for all non-negative integers $m$ as follows:

$$Q_m(s,a) = R(s,a) + \gamma \sum_{s' \in S} [T(s,a,s') \max_{a' \in A} Q_{m-1}(s',a')]. \tag{3}$$

where we set $Q_{-1}(s',a') = 0$. We then define the $V_m(s)$ as:

$$V_m(s') = \max_{a' \in A} Q_m(s',a').$$

We can rewrite the equation $Q_m(s,a)$ as follows:

$$Q_m(s,a) = R(s,a) + \gamma \sum_{s' \in S} [T(s,a,s') V_{m-1}(s')].$$

For the base case of $m = 0$, we have

$$\begin{aligned} Q_0(s,a) &= R(s,a) \\ &= R(L_g[s], K_g[a]) \\ &= Q_0(L_g[s], K_g[a]). \end{aligned}$$

* Rongye Shi. Email: shirongye@buaa.edu.cn

As we have the base case, let's assume that $Q_j(s,a) = Q_j(L_g[s], K_g[a])$ holds for all $j < m$ and all state-action pairs $(s,a) \in \Psi$. It follows that:

$$\max_{a \in A} Q_j(s,a) = \max_{a \in A} Q_j(L_g[s], K_g[a]),$$

which implies:

$$V_j(s) = V_j(L_g[s]). \tag{4}$$

Now we prove by induction on $m$ that the theorem is true. For the case m, we have:

$$\begin{aligned} Q_m(s,a) &= R(s,a) + \gamma \sum_{s' \in S} T(s,a,s') V_{m-1}(s') \\ &= R(L_g[s], K_g[a]) + \gamma \sum_{s' \in S} T(L_g[s], K_g[a], L_g[s']) V_{m-1}(s'). \end{aligned} \tag{5}$$

Let's define:

$$F = \gamma \sum_{s' \in S} T(L_g[s], K_g[a], L_g[s'])) V_{m-1}(s').$$

Then, by substituting Equation (4) into $F$, we obtain:

$$F = \gamma \sum_{s' \in S} T(L_g[s], K_g[a], L_g[s'])) V_{m-1}(L_g[s']).$$

Substituting $F$ back to equation (5), we get:

$$Q_m(s,a) = Q_m(L_g[s], K_g[a]). \tag{6}$$

Equation (6) shows $Q_m(s,a) = Q_m(L_g[s], K_g[a])$ for all non-negative integers $m$ via induction. The optimal action-value function $Q^*(s,a)$, the limit of $Q_m(s,a)$ as $m$ approaches infinity, also follows this property due to bounded rewards. Then we have:

$$Q^\star(s,a) = Q^\star(L_g[s], K_g[a]),$$

$$V^\star(s) = V^\star(L_g[s]).$$

Therefore, by mathematical induction, the proposition 1 is true. □

The boundedness of the reward function is important for ensuring that the limit exists. The action-value function $Q_m(s,a)$ is computed recursively and involves summing up rewards. If the rewards weren't bounded, then these sums could potentially become infinite, and the limit as $m$ goes to infinity wouldn't exist.

## 2 Examining Data Augmentation Implementation

While data augmentation has been previously utilized in RL, we argue that there are practical issues with its application. To illustrate this, we will analyze the implementation of data augmentation in several parts of equation (7).

In the default formulation of MAPPO under the Dec-POMDP framework, the agents employ the trick of policy sharing. As such, the MAPPO learns policy $\pi_\theta$ by optimizing the following objective:

$$J_\pi(\theta)=\sum_{i=1}^{n} E_{\pi_{\theta_{\text{old}}}}\left[\frac{\pi_\theta\left(a^i \mid s\right)}{\pi_{\theta_{\text{old}}}\left(a^i \mid s\right)} A^\pi\left(s, a^i\right)\right], \tag{7}$$

where $\pi_{\theta_{\text{old}}}$ is the behavior policy used to collect trajectories, $\pi_\theta$ is the policy we want to optimize, and $A^\pi\left(s, a^i\right)$ denotes the advantage function.

The implementation of each part in equation (7) during the training of agents is as follows: 1)The numerator of the first term in equation (7) is calculated using the latest policy $\pi$ and the samples obtained from the replay buffer. If the sampled data is an augmented sample, i.e., $(L_g[s], K_g[a])$, then this term is $\pi_\theta(K_g[a] \mid L_g[s])$. 2)The denominator is calculated using the state-action pair $(s, a)$ and the old policy $\pi_{\theta_{old}}$, because we can only interact with the environment through real observations and not augmented ones. This term is stored in the replay buffer during the interaction of the agent with the environment, so it is $\pi_{\theta_{old}}(K_g[a] \mid L_g[s])$. 3)The second term $A$ in equation (7) is calculated using the rewards generated during the interaction. Therefore, this term is still based on the original samples, i.e., $A_\psi^\pi\left(s, a^i\right)$.

Thus, If transformation $(L_g, K_g)$ is applied to the algorithm, the MAPPO objective changes, and equation (7) is replaced by (8). It is worth noting that depending on the specific data augmentation method used, there may be minor differences in the details, but most papers that use data augmentation follow this approach[3]. Even if transforming both the numerator and denominator distributions depending on the exact implementation would result in a larger variance, which is also unreasonable.

$$J_\pi(\theta)=\sum_{i=1}^{n} E_{\pi_{\theta_{\text{old}}}}\left[\frac{\pi_\theta\left(K_g[a^i] \mid L_g[s]\right)}{\pi_{\theta_{\text{old}}}\left(a^i \mid s\right)} A_\psi^\pi\left(s, a^i\right)\right]. \tag{8}$$

A certain transformation $(L_g, K_g)$ for data augmentation can result in an arbitrarily large ratio $\pi_\theta(K_g[a] \mid L_g[s])/\pi_{\theta_{old}}(a \mid s)$. In multi-agent settings, when multiple agents are considered, more sources of variance are introduced, making the training severely unstable as shown in equation (8).

## 3 Symmetric Transformation

The most general form of symmetry in multi-agent systems is the global symmetry depicted in Figure 1, where rotating the global state leads to a permutation of the optimal joint policy. When a problem is characterized as a Symmetric Markov Game, it inherently exhibits this symmetry. It is important to note that the optimal policy can be expressed in terms of the optimal Q-function since the optimal action at a given state is the one that maximizes the Q-function at that state. As a result, the assertion made in Figure 1 is substantiated: a global state rotation yields a permutation of the optimal joint policy. This outcome is a direct implication of the optimal Q-function equivalence, as stated in Proposition 1. We describe the specific details of symmetry transformation by taking the cooperative navigation shown in Figure 1 as an example. We consider rotation transformation in the 2D space that is the set of 90 degree rotations $\{0^\circ, 90^\circ, 180^\circ, 270^\circ\}$.

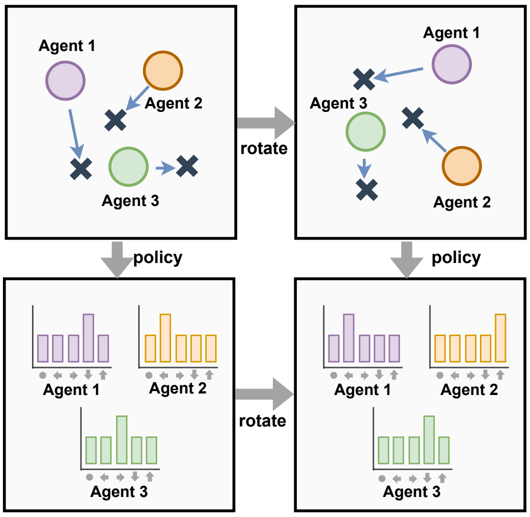


**Figure 1**: Rotating the state globally in the cooperative navigation task results in a permutation of the optimal joint policy.

## 4 ESP for Dec-POMDPs with symmetry

Our framework ESP is based on data augmentation and is not limited by fully observable or partial observable. The method can be applied to a wide range of problems, including those modeled as Markov games and Dec-POMDPs.

**Dec-POMDP**.A fully cooperative multi-agent task can be formalized as a decentralized partially-observable Markov decision process (Dec-POMDP) consisting of a tuple $(N, S, \{A_i\}_{i=1}^n, \{O_i\}_{i=1}^n, R, T, \{U_i\}_{i=1}^n, \gamma)$ [6]. $N, S, \{A_i\}_{i=1}^n, \{O_i\}_{i=1}^n$ denote the set of states, agents, actions and observations, respectively, where a subscript $i$ represents the set pertaining to agent $i \in \mathcal{N} = \{1, \ldots, n\}$. We also write $A = \times_i A^i$ and $O = \times_i O^i$, the sets of joint actions and observations, respectively. $s_t \in S$ is the state at time $t$. $a_t \in A$ is the joint action of all agents taken at time $t$, which changes the state according to the transition distribution $s_{t+1} \sim T\left(s_{t+1} \mid s_t, a_t\right)$. The subsequent joint observation of the agents is $o_{t+1} \in O$, according to $o_{t+1} \sim U\left(o_{t+1} \mid s_{t+1}, a_t\right)$, where $U = \times_i U^i$. The reward $r_{t+1} \in R$ is according to the reward function. $\gamma \in [0, 1]$ is the discount factor. Notating $\tau_t^i = \left(a_0^i, o_1^i, \ldots, a_{t-1}^i, o_t^i\right)$ for the action-observation history of agent $i$, agent $i$ acts according to a policy $a_t^i \sim \pi^i\left(a_t^i \mid \tau_t^i\right)$. The agents seek to maximize the expected discounted sum of rewards.

**Dec-POMDPs with symmetry**. We propose Dec-POMDPs with symmetry which is a subclass of the Dec-POMDPs endowed with symmetry characterization. The Dec-POMDPs with symmetry $(N, S, \{A_i\}_{i=1}^n, \{O_i\}_{i=1}^n, R, T, \{U_i\}_{i=1}^n, \gamma, G)$ is a Dec-POMDPs that satisfies the conditions of policy equivalence and value invariance. The observation transformation and action transformation in the Dec-POMDPs with symmetry are defined as $L_g$ and $K_g$, respectively. We use $\phi$ to represent symmetric transformations of the trajectory. $\phi$ acts on the action-observation history as

$$\phi\left(\tau_t^i\right)=\left(K_g\left(a_0^i\right), L_g\left(o_1^i\right), \ldots, K_g\left(a_{t-1}^i\right), L_g\left(o_t^i\right)\right).$$

Further, for all $g \in G$, and for all $\tau$, the conditions of policy equivalence and value invariance are given by:

$$V(\tau) = V(\phi[\tau]), \tag{9}$$

$$\pi(a \mid \tau) = \pi(K_g(a) \mid \phi[\tau]). \tag{10}$$

Our method focuses on systems with global symmetry. As depicted in Figure 2, when the global state is rotated, the corresponding local observation also rotates. when facing partially observable problems, by utilizing the rotation transformation represented by $\phi$, we are able to rotate the observation-action pairs. A summary of the training procedure of our ESP framework for Dec-POMDPs is described in Algorithm 1. We start by initializing the group transformation $h = (L_g, K_g)$ alongside several training parameters, including agent numbers, maximum steps, batch size. Then the transformation $h = (L_g, K_g)$ is selected according to the group $g$. After that, the real trajectories generated by agents are augmented by symmetric transformation. Both real and augmented samples are stored in an experience replay buffer. Finally, data is sampled from the experience replay buffer to update the agent network. In the execution phase, the agents can perform the policies in a distributed manner. The symmetry consistency loss for the policy and value function in Dec-POMDPs is defined as:

$$S_\pi = KL\left[\pi_\theta(K_g[a] \mid \phi[\tau]) \mid \pi_\theta(a \mid \tau)\right], \tag{11}$$

$$S_V = E_\pi\left[(V_\psi(\tau) - V_\psi(\phi[\tau]))^2\right]. \tag{12}$$

**Symmetric transformation for observation.** In this task, agents need to simultaneously cover three target locations in a 2D space whilst avoiding collisions with each other. Agents observe the relative positions of other agents and landmarks and decide to move. The state of agent $i$ is represented through *self velocity*, *self position*, *landmark relevant positions*, and *other agent relevant positions*. When performing a rotation operation on a state, we can multiply each element by the rotation matrix. The element of state such as *self velocity* can be represented by a vector $(V_x, V_y)$. We apply rotation to generate the new velocity as shown in equation (13).

$$L_g[V_x, V_y] = [V_x, V_y] \cdot \begin{bmatrix} \cos\theta & -\sin\theta \\ \sin\theta & \cos\theta \end{bmatrix} \tag{13}$$

**Symmetric transformation for action.** In the discrete action spaces, the action of the agent is denoted as a one-hot vector as *no action*, *left*, *right*, *down*, *up*. A transformation $K_g$ acting on the action is represented as a matrix multiplication of the action vector with a permutation matrix. Take the action vector $[0, 0, 1, 0, 0]$ of turning right as an example. The way to apply rotation to generate a new action is shown in (14) where $P$ is the permutation matrix.

$$\begin{aligned} K_g[a] &= [0, 0, 1, 0, 0] \cdot P \\ &= [0, 0, 0, 1, 0] \end{aligned} \tag{14}$$

## 5 Information About Task

In this section, we present the experimental details of the formation change task for multiple robots, which was inspired by [2]. We define the observation space, action space, and reward function as follows.

**Observation space**. The observation of each robot is the concatenation of its velocity direction and the relative coordinates of the others in the environment. As shown in figure 3, the observation of the robot can be denoted as :

$$(\theta_i, dx_1, dy_1, dx_2, dy_2, dx_3, dy_3),$$

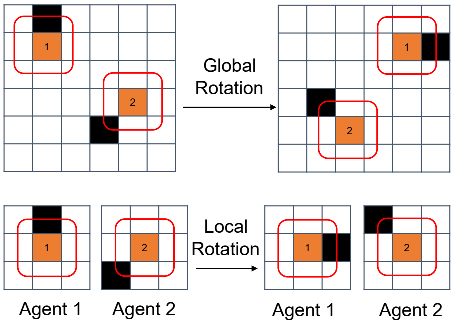


**Figure 2**: The relationship between global transformation and local transformation.

**Algorithm 1** Exploiting Symmetry Prior for Multi-Agent Reinforcement Learning with respect to Dec-POMDPs

**Input:** Transformation $L_g$, $K_g$ and $\phi$. $g \in G$

Initialize agent number $N$, max steps in an episode $T_e$, replay buffer $\mathcal{D}$ and the episode batch size $M$
Initialize $\theta$ and $\Psi$, the parameters for policy and critic
**for** each episode **do**
  **for** t=1 to $T_e$ **do**
    for each agent i, select action $a_i$ w.r.t the policy
    Execute actions $a = (a_1, \ldots, a_N)$ and Collect trajectories $\tau$
    $\hat{\tau} \longleftarrow \phi(\tau)$
    Store $\tau$ and $\hat{\tau}$ to the replay buffer $\mathcal{B}$
  **end for**
  **if** *episodes* $> M$ **then**
    Sample a minibatch $\mathcal{B} = \{\tau^j\}_{j=0}^{M} \sim \mathcal{D}$
    Calculate the symmetry consistency loss using Equation (11) or (12)
    Update the parameters $\theta$ of the policy network
    Update the parameters $\Psi$ of the critic network
  **end if**
**end for**

where $\theta_i$ is the velocity direction of agent $i$. And the$(dx, dy)$indicates the relative coordinates of the others in the environment. The subscript $i$ represents the nearest obstacle, goal, and agents when equals 1,2,3 respectively.

**Action space**. We choose Epuck as the robot model in the Webots simulator. Agents can assign the two wheel-speed to control the robot. And the wheel speed are range from $-1$ to 1.

**Reward function**. For each agent $i \in I$ we define a term for reaching the goal position and for avoiding collisions each by Equation (15) with desired target position $g_i \in R^2$, avoidance radius $C \geq 0$. The coordination of the agent $i$ and the obstacle $j$ at step $t$ is denoted as $p_i^t$ and $c_j$.

$$r_i^t = g_i^t + c_i^t. \tag{15}$$

The $g_i^t$ and $c_i^t$ were defined as:

$$g_i^t = \omega_g\left(\left\|\mathrm{p}_i^{t-1} - \mathrm{g}_i\right\| - \left\|\mathrm{p}_i^t - \mathrm{g}_i\right\|\right). \tag{16}$$

The $c_i^t$ were defined as:

$$c_i^t = \begin{cases} c_{\text{collision}} & \text{if } \left\|\mathrm{p}_i^t - \mathrm{c}_j\right\| < C \\ 0 & \text{otherwise} \end{cases}. \tag{17}$$

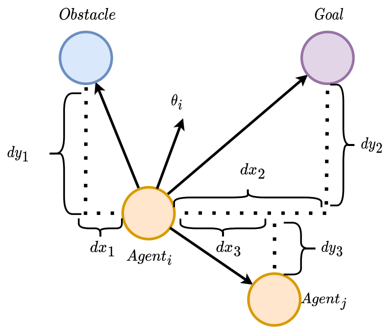


**Figure 3**: The observation space of the agents in formation change.

The parameters of the reward function are denoted as below: $r_{arrival} = 0.05, \omega_g = 100, c_{collision} = 0.35, C = 0.5$.

For the cooperative navigation and predator-prey tasks, the description of the state and action spaces, as well as the reward functions, can be found in the pettingzoo library website: https://pettingzoo.farama.org/environments/mpe/.

## 6 Physical Deployment

For real-world scenarios, we believe that absolute coordinates are part of the agents' inputs, and ESP can be beneficial for performance improvement. We performed physical experiments on a set of e-puck2 robots, a widely used mini mobile robot developed by EPFL in various research and educational scenarios [5]. To increase their computing power, we added an expansion board with Raspberry Pi, as shown in Figure 4 and 5. The pi-puck extension, which consists of a Raspberry Pi Zero W and adapter PCB, was directly connected to the onboard MCU and sensors for interaction [4]. We installed ROS2 on the Raspberry Pi Zero W, and the deep neural network was used to control the physical robot [8]. The experiments took place in a 2m $\times$ 2m indoor arena with walls on the boundary, and a centralized motion capture system was added to capture the position of each robot. We used a motion capture system that provides absolute coordinates, allowing the e-puck to benefit from the ESP. This allowed us to calculate the state and observation information required by the policy [7].

To make the experiments easy to implement, we removed the obstacles introduced in section 6.1. We have integrated our ESP approach into the MAPPO algorithm, which has resulted in a reduction in the number of risky states encountered by the agents during task completion. Risky states refer to those states in which the distance between agents is less than 5 centimeters, and the rate of risky states is calculated as the proportion of such states to all states. In comparison to the MAPPO algorithm, the ESP-MAPPO algorithm has demonstrated a lower rate of risky states, with only 2.2% of states being classified as risky, while the rate for MAPPO is higher at 5.8%. For further information and visual demonstrations of the findings, please refer to the supplementary materials, which include detailed videos.

## 7 Hyperparameters And Experimental Details

For clarity of presentation, the MADDPG is used as an example to introduce the symmetry consistency loss for a value-based algorithm. The MADDPG adapts the centralized training with decentralized execution (CTDE) framework. The centralized action-value function

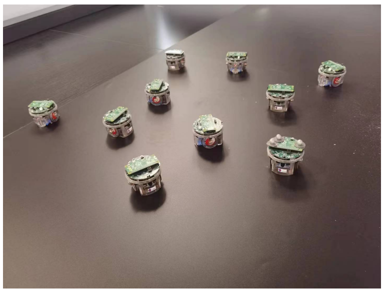

**Figure 4**: The Epuck robots for formation change task.

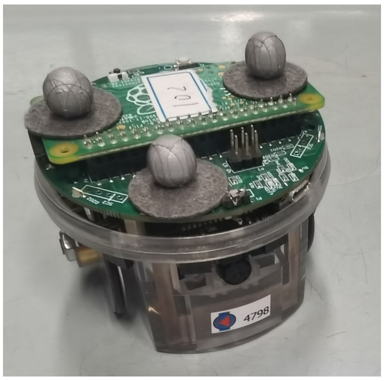

**Figure 5**: The real Epuck with pi-puck extension.

$Q_i^{\mu}$ is updated by:

$$S_{MADDPG}(\phi) = E_{s,a}\left[\left(Q\left(s, a_1, \ldots, a_N\right) - y\right)^2\right] \tag{18}$$

where $y = r + \gamma Q(s', a'_1, \ldots, a'_N)$ and $a'_j$ is obtained by the current policy; $Q_\phi(s, a)$ represent the Q-value under the original state input, and $Q_\phi(L_g[s], K_g^s[a])$ to represent the Q-value under symmetry state input where $a$ indicates the joint action of all agents. Then, the square of $L_2$ distance between the Q-network outputs under the original state, and the symmetric transformed state can be directly calculated by:

$$S_{MADDPG}\left(\phi\right) = E_{s,a}\left[\left(Q_\phi(s, a) - Q_\phi(L_g[s], K_g^s[a])\right)^2\right]. \tag{19}$$

This item can help constrain the agent's value function to satisfy the defined symmetry constraints.

In all our scenarios, the hyperparameters used the default parameters from paper [11]. Tables 2 describe the hyperparameters for MAPPO. For ESP, each interaction sample along with its augmented ones will be added all together to the buffer at each time step. We used the same buffer size for both ESP and non-ESP across all experiments.

Table 3 describe the hyperparameters for the QMix, and MADDPG. We utilize parameter sharing when there are homogenous agents because this has been the accepted practice in the majority of past MARL works [10, 1, 9]. To train the QMIX algorithm in the formation change task, the continuous action space were discretized into a finite set of atomic actions and reduce the original task into a new task with a discrete action space. For a continuous action space of -1 to 1, the action space were discretized every 0.2. The computational experiments were performed on a Linux server with an i9-12900KF CPU. The Python version used was 3.9.12, and the PyTorch version used was 1.13.0.

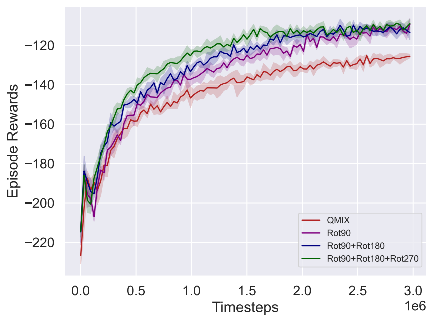


(a) Learning curve of QMIX using augmentation solely with different numbers.

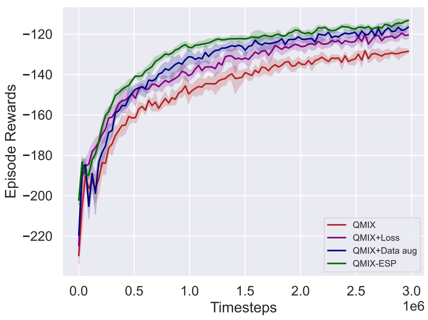


(b) Learning curve of four variants of QMIX in the task.

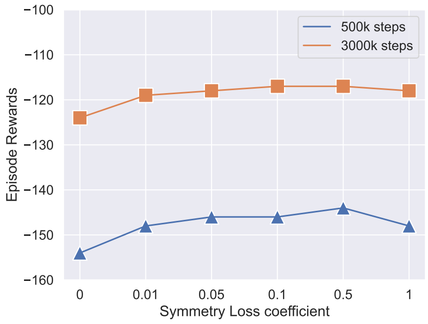


(c) Parameter sensitivity of coefficient at different training steps of QMIX.

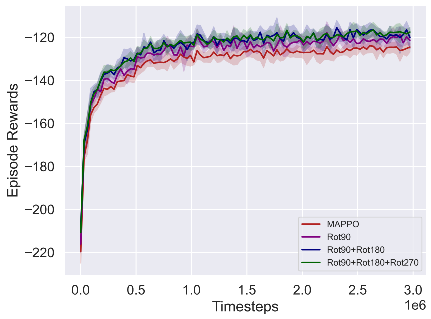


(d) Learning curve of MAPPO using augmentation solely with different numbers.

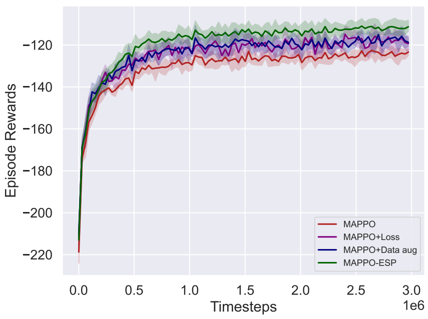


(e) Learning curve of four variants of MAPPO in the task.

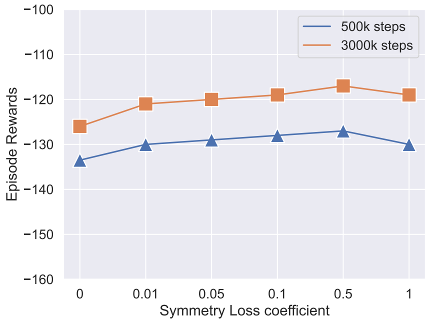


(f) Parameter sensitivity of coefficient at different training steps of MAPPO.

**Figure 6**: The ablation study and parameter sensitivity of our ESP framework for QMIX and MAPPO.

**Table 1**: Episode rewards of the ESP and baselines on the CN task; '500k' and '3000k' represent the number of training steps of the algorithms. 'N' represents the number of agents. The error bars are the standard error of the mean.

| Agent | Step | MADDPG | MADDPG-ESP | QMIX | QMIX-ESP | MAPPO | MAPPO-ESP |
|---|---|---|---|---|---|---|---|
| N=2 | 500K | -101.42±3.24 | -94.12±2.15 | -106.65±3.68. | -98.75±1.89 | -99.12±3.25 | -92.68±2.65 |
| | 3000K | -95.72±1.25 | -90.92±2.54 | -95.95±2.42 | -89.32±2.31 | -94.67±1.87 | -87.54±2.56 |
| N=3 | 500k | -145.23±3.71 | -132.22±1.27 | -154.24±3.16 | -140.12±2.25 | -132.65±2.89 | -122.25±1.62 |
| | 3000k | -122.63±6.04 | -112.21±2.75 | -124.67±3.05 | -113.84±1.43 | -126.97±2.12 | -110.22±2.12 |
| N=4 | 500K | -187.57±4.12 | -179.93±5.24 | -192.57±4.23 | -186.32±3.14 | -189.42±4.52 | -183.87±3.24 |
| | 3000K | -183.43±4.68 | -178.62±5.12 | -191.57±4.24 | -185.92±3.65 | -187.73±2.45 | -182.81±2.98 |

**Table 2**: hyperparameters used in MAPPO.

| Hyperparameters | value |
|---|---|
| recurrent data chunk length | 10 |
| gradient clip norm | 10.0 |
| gae lamda | 0.95 |
| gamma | 0.99 |
| value loss | huber loss |
| huber delta | 10.0 |
| batch size | buffer length × num agents |
| mini batch size | batch size / mini-batch |
| optimizer | Adam |
| optimizer epsilon | 1e-5 |
| weight decay | 0 |
| network initialization | Orthogonal |
| use reward normalization | True |
| use feature normalization | True |

**Table 3**: Hyperparameters used in QMix and MADDPG.

| Hyperparameters | Value |
|---|---|
| Gradient clip norm | 10.0 |
| Random episodes | 5 |
| Epsilon | 1->0.05 |
| Epsilon anneal time | 50000 timesteps |
| Train interval | 1 episode |
| Gamma | 0.99 |
| Buffer size | 5000 episodes |
| Batch size | 32 episodes |
| Optimizer eps | 1e-5 |
| Optimizer | Adam |
| Weight decay | 0 |
| Network initialization | Orthogonal |
| Use reward normalization | True |
| Use feature normalization | True |

## 8 Additional Experimental Details

We extended the ablation experiments in the main text to QMIX and MAPPO algorithms, as shown in Figure 6. To examine the impact of the number of agents on our ESP, we conducted experiments on the cumulative discounted reward under different numbers of agents, as shown in Table 1. It can be observed that our method is effective for various numbers of agents.

## References


[1] Filippos Christianos, Georgios Papoudakis, Muhammad A Rahman, and Stefano V Albrecht, 'Scaling multi-agent reinforcement learning with selective parameter sharing', in *International Conference on Machine Learning*, pp. 1989–1998. PMLR, (2021).

[2] Tingxiang Fan, Pinxin Long, Wenxi Liu, and Jia Pan, 'Distributed multi-robot collision avoidance via deep reinforcement learning for navigation in complex scenarios', *The International Journal of Robotics Research*, **39**(7), 856–892, (2020).

[3] Misha Laskin, Kimin Lee, Adam Stooke, Lerrel Pinto, Pieter Abbeel, and Aravind Srinivas, 'Reinforcement learning with augmented data', *Advances in Neural Information Processing Systems*, **33**, (2020).

[4] Alan G Millard, Russell Joyce, James A Hilder, Cristian Fleşeriu, Leonard Newbrook, Wei Li, Liam J McDaid, and David M Halliday, 'The Pi-puck extension board: a raspberry pi interface for the E-puck robot platform', in *2017 IEEE/RSJ International Conference on Intelligent Robots and Systems (IROS)*, pp. 741–748. IEEE, (2017).

[5] Francesco Mondada, Michael Bonani, Xavier Raemy, James Pugh, Christopher Cianci, Adam Klaptocz, Stephane Magnenat, Jean-Christophe Zufferey, Dario Floreano, and Alcherio Martinoli, 'The E-puck, a robot designed for education in engineering', in *Proceedings of the 9th conference on autonomous robot systems and competitions*, volume 1, pp. 59–65. IPCB: Instituto Politécnico de Castelo Branco, (2009).

[6] Frans A Oliehoek and Christopher Amato, *A concise introduction to decentralized POMDPs*, Springer, 2016.

[7] Alexandra Pfister, Alexandre M West, Shaw Bronner, and Jack Adam Noah, 'Comparative abilities of microsoft kinect and vicon 3d motion capture for gait analysis', *Journal of medical engineering & technology*, **38**(5), 274–280, (2014).

[8] Morgan Quigley, Ken Conley, Brian Gerkey, Josh Faust, Tully Foote, Jeremy Leibs, Rob Wheeler, Andrew Y Ng, et al., 'Ros: an open-source robot operating system', in *ICRA workshop on open source software*, volume 3, p. 5. Kobe, Japan, (2009).

[9] Tabish Rashid, Mikayel Samvelyan, Christian Schroeder, Gregory Farquhar, Jakob Foerster, and Shimon Whiteson, 'QMIX: Monotonic value function factorisation for deep multi-agent reinforcement learning', in *International Conference on Machine Learning*, pp. 4295–4304. PMLR, (2018).

[10] Tonghan Wang, Tarun Gupta, Anuj Mahajan, Bei Peng, Shimon Whiteson, and Chongjie Zhang, 'Rode: Learning roles to decompose multi-agent tasks', in *International Conference on Learning Representations*.

[11] Chao Yu, Akash Velu, Eugene Vinitsky, Yu Wang, Alexandre Bayen, and Yi Wu, 'The surprising effectiveness of PPO in cooperative, multi-agent games', *arXiv preprint arXiv:2103.01955*, (2021).
